# Supplementary material for: A Systematic Review on Custom Data Gloves
Source: arXiv:2405.15417 ancillary file (2024-05-24)
Supplement: Supplementary file 1 [file Data_Glove_Review2_Table.pdf]

# A Systematic Review on Custom Data Gloves

Valerio Belcamino, Alessandro Carfi, Fulvio Mastrogiovanni

TABLE I: The table contains the results of the classification described in this publication, sensor type, DoFs, palm area covered by pressure sensors (in  $\text{cm}^2$ ), and, finally, the classification in application fields.

| Author                    | Year | IMU | Flex | Pressure | Magnetic | DoFs    | P. Area ( $\text{cm}^2$ ) | Application               |
|---------------------------|------|-----|------|----------|----------|---------|---------------------------|---------------------------|
| Rand et al. [1]           | 1993 |     | 1    |          |          | [0,5]   |                           | None                      |
| Karlsson et al. [2]       | 1998 |     | 1    |          |          | [0,5]   |                           | Human-Machine Interaction |
| Crook et al. [3]          | 1998 |     |      | 1        |          |         | 6,78                      | Functionality Assessment  |
| You et al. [4]            | 2001 |     | 1    |          |          | [11,18] |                           | Human-Machine Interaction |
| Bouzit et al. [5]         | 2002 |     |      |          | 1        | [0,5]   |                           | Human-Machine Interaction |
| Mazzoldi et al. [6]       | 2002 |     | 1    |          |          | [19+]   |                           | Functionality Assessment  |
| Tarchanidis et al. [7]    | 2003 |     | 1    | 1        |          | [0,5]   | 0,65                      | Environment Interaction   |
| Su et al. [8]             | 2003 |     |      |          | 1        | [19+]   |                           | Functionality Assessment  |
| Ku et al. [9]             | 2003 |     | 1    |          |          | [0,5]   |                           | Functionality Assessment  |
| Mraz et al. [10]          | 2003 |     | 1    |          |          | [0,5]   |                           | Human-Machine Interaction |
| Fahn et al. [11]          | 2005 |     |      |          | 1        | [11,18] |                           | Environment Interaction   |
| Bao et al. [12]           | 2006 |     | 1    | 1        |          | [11,18] |                           | Human-Machine Interaction |
| Bui et al. [13]           | 2007 | 1   |      |          |          | [11,18] |                           | Human-Machine Interaction |
| Su et al. [14]            | 2007 |     |      |          | 1        | [11,18] |                           | None                      |
| Komi et al. [15]          | 2008 |     |      | 1        |          |         | 12,56                     | Environment Interaction   |
| Amirouche et al. [16]     | 2008 |     | 1    | 1        |          | [0,5]   | 0,79                      | Environment Interaction   |
| King et al. [17]          | 2009 | 1   | 1    |          |          | [11,18] |                           | Environment Interaction   |
| Maréchal et al. [18]      | 2009 |     |      | 1        |          |         | 1,80                      | Functionality Assessment  |
| Fu et al. [19]            | 2009 |     | 1    |          |          | [0,5]   |                           | Human-Machine Interaction |
| Fahn et al. [20]          | 2010 |     |      |          | 1        | [11,18] |                           | None                      |
| Gallo et al. [21]         | 2010 | 1   | 1    |          |          | [6,10]  |                           | Human-Machine Interaction |
| Fu et al. [22]            | 2010 |     | 1    |          |          | [0,5]   |                           | Human-Machine Interaction |
| Wang et al. [23]          | 2010 |     | 1    |          |          | [6,10]  |                           | Environment Interaction   |
| Da Silva et al. [24]      | 2011 |     | 1    |          |          | [11,18] |                           | Human-Machine Interaction |
| Dalley et al. [25]        | 2012 |     | 1    |          |          | [0,5]   |                           | Human-Machine Interaction |
| Falco et al. [26]         | 2012 |     | 1    |          |          | [11,18] |                           | Environment Interaction   |
| Fujiwara et al. [27]      | 2013 |     | 1    |          |          | [0,5]   |                           | Human-Machine Interaction |
| Tongrod et al. [28]       | 2013 |     | 1    | 1        |          | [6,10]  | 10,70                     | Human-Machine Interaction |
| Fujiwara et al. [29]      | 2014 |     | 1    |          |          | [0,5]   |                           | Environment Interaction   |
| Yuen et al. [30]          | 2014 |     | 1    |          |          | [0,5]   |                           | None                      |
| Tanaka et al. [31]        | 2014 |     | 1    |          |          | [0,5]   |                           | Functionality Assessment  |
| Shukor et al. [32]        | 2015 | 1   |      |          |          | [6,10]  |                           | Human-Machine Interaction |
| Schuster-Amft et al. [33] | 2015 | 1   | 1    |          |          | [6,10]  |                           | Functionality Assessment  |
| Kim et al. [34]           | 2015 | 1   |      |          |          | [11,18] |                           | Human-Machine Interaction |
| Chen et al. [35]          | 2015 |     | 1    |          |          | [0,5]   |                           | Human-Machine Interaction |
| Girovský et al. [36]      | 2015 | 1   | 1    |          |          | [6,10]  |                           | Human-Machine Interaction |
| Saini et al. [37]         | 2015 |     | 1    |          |          | [0,5]   |                           | Human-Machine Interaction |
| Galka et al. [38]         | 2016 | 1   |      |          |          | [11,18] |                           | Human-Machine Interaction |
| Li et al. [39]            | 2016 | 1   |      |          |          | [19+]   |                           | Human-Machine Interaction |
| Lorussi et al. [40]       | 2016 | 1   | 1    | 1        |          | [6,10]  | 3,93                      | Functionality Assessment  |
| Liu et al. [41]           | 2016 |     | 1    |          |          | [0,5]   |                           | Human-Machine Interaction |
| Kim et al. [42]           | 2016 |     | 1    |          |          | [0,5]   |                           | Environment Interaction   |
| Tavares et al. [43]       | 2016 | 1   | 1    | 1        |          | [11,18] |                           | Functionality Assessment  |
| Che-Ani et al. [44]       | 2016 |     | 1    |          |          | [0,5]   |                           | Environment Interaction   |
| El Hoda Saleh et al. [45] | 2016 |     | 1    |          |          | [0,5]   |                           | Functionality Assessment  |
| Yahya et al. [46]         | 2017 |     | 1    |          |          | [0,5]   |                           | Human-Machine Interaction |
| Lin et al. [47]           | 2017 | 1   |      |          |          | [19+]   |                           | Functionality Assessment  |
| Zuruzi et al. [48]        | 2017 |     |      | 1        |          |         | 4,00                      | None                      |
| Fang et al. [49]          | 2017 | 1   |      |          |          | [19+]   |                           | Human-Machine Interaction |
| Lin et al. [50]           | 2017 |     | 1    | 1        |          | [0,5]   | 0,79                      | Human-Machine Interaction |
| Asadipour et al. [51]     | 2017 |     |      | 1        |          |         | 16,10                     | Functionality Assessment  |

TABLE I: The table contains the results of the classification described in this publication - continued.

| Author                       | Year | IMU | Flex | Pressure | Magnetic | DoFs    | P. Area (cm <sup>2</sup> ) | Application               |
|------------------------------|------|-----|------|----------|----------|---------|----------------------------|---------------------------|
| Ganjdanesh et al. [52]       | 2017 | 1   |      |          |          | [19+]   |                            | Human-Machine Interaction |
| Connolly et al. [53]         | 2018 | 1   |      |          |          | [19+]   |                            | Functionality Assessment  |
| Lin et al. [54]              | 2018 | 1   |      |          |          | [19+]   |                            | Functionality Assessment  |
| Mummadi et al. [55]          | 2018 | 1   |      |          |          | [6,10]  |                            | Human-Machine Interaction |
| Liao et al. [56]             | 2018 |     |      | 1        |          |         | 5,00                       | Human-Machine Interaction |
| Lu et al. [57]               | 2018 |     | 1    |          |          | [0,5]   |                            | Human-Machine Interaction |
| Choi et al. [58]             | 2018 | 1   |      |          |          | [19+]   |                            | Environment Interaction   |
| Kanokoda et al. [59]         | 2018 |     | 1    |          |          | [0,5]   |                            | Human-Machine Interaction |
| Saldaña González et al. [60] | 2018 | 1   |      |          |          | [0,5]   |                            | Human-Machine Interaction |
| Shahrampour et al. [61]      | 2018 |     |      | 1        |          |         |                            | Environment Interaction   |
| Hoda et al. [62]             | 2018 |     |      | 1        |          |         | 7,65                       | Functionality Assessment  |
| Kao et al. [63]              | 2018 | 1   | 1    | 1        |          | [11,18] |                            | Environment Interaction   |
| Malawski et al. [64]         | 2018 | 1   |      |          |          | [6,10]  |                            | Human-Machine Interaction |
| Chacon et al. [65]           | 2018 |     | 1    |          |          | [6,10]  |                            | Environment Interaction   |
| Javaid et al. [66]           | 2018 | 1   |      | 1        |          | [0,5]   | 13,34                      | Environment Interaction   |
| Glauser et al. [67]          | 2019 |     | 1    |          |          | [19+]   |                            | Human-Machine Interaction |
| Zhang et al. [68]            | 2019 |     | 1    |          |          | [0,5]   |                            | None                      |
| Zhang et al. [69]            | 2019 |     |      | 1        |          | [0,5]   |                            | Human-Machine Interaction |
| Huang et al. [70]            | 2019 |     | 1    |          |          | [6,10]  |                            | Human-Machine Interaction |
| Lin et al. [71]              | 2019 | 1   |      |          |          | [19+]   |                            | Functionality Assessment  |
| Stornelli et al. [72]        | 2019 | 1   | 1    |          |          | [11,18] |                            | Functionality Assessment  |
| Kim et al. [73]              | 2019 |     | 1    |          |          | [0,5]   |                            | Human-Machine Interaction |
| Lin et al. [74]              | 2019 | 1   |      |          |          | [19+]   |                            | Functionality Assessment  |
| Mehra et al. [75]            | 2019 | 1   | 1    |          |          | [6,10]  |                            | Human-Machine Interaction |
| Chuang et al. [76]           | 2019 |     | 1    |          |          | [0,5]   |                            | Human-Machine Interaction |
| Jiang et al. [77]            | 2019 | 1   |      |          |          | [11,18] |                            | Environment Interaction   |
| Li et al. [78]               | 2019 | 1   | 1    |          |          | [6,10]  |                            | Human-Machine Interaction |
| Liu et al. [79]              | 2019 | 1   |      |          |          | [6,10]  |                            | Environment Interaction   |
| Melnyk et al. [80]           | 2019 | 1   |      | 1        |          | [0,5]   |                            | Environment Interaction   |
| Minh et al. [81]             | 2019 | 1   |      |          |          | [19+]   |                            | None                      |
| Ullah et al. [82]            | 2019 | 1   |      |          |          | [0,5]   |                            | Human-Machine Interaction |
| Yao et al. [83]              | 2019 |     |      | 1        |          |         | 172,00                     | Environment Interaction   |
| Umar et al. [84]             | 2019 | 1   |      |          |          | [0,5]   |                            | Functionality Assessment  |
| Zhang et al. [85]            | 2019 |     | 1    |          |          | [6,10]  |                            | Human-Machine Interaction |
| Lim et al. [86]              | 2019 | 1   |      |          |          | [0,5]   |                            | Environment Interaction   |
| Puasa et al. [87]            | 2019 | 1   | 1    | 1        |          | [6,10]  |                            | Human-Machine Interaction |
| Shwetha et al. [88]          | 2019 | 1   | 1    |          |          | [0,5]   |                            | Human-Machine Interaction |
| Syed Mubarak Ali et al. [89] | 2019 |     | 1    |          |          | [0,5]   |                            | Human-Machine Interaction |
| Abtahi et al. [90]           | 2020 |     | 1    |          |          | [0,5]   |                            | Functionality Assessment  |
| Song et al. [91]             | 2020 |     | 1    |          |          | [0,5]   |                            | None                      |
| Zhang et al. [92]            | 2020 |     | 1    |          |          | [0,5]   |                            | None                      |
| Chang et al. [93]            | 2020 | 1   |      |          |          | [19+]   |                            | Human-Machine Interaction |
| Hang et al. [94]             | 2020 |     | 1    |          |          | [0,5]   |                            | Human-Machine Interaction |
| Zhang et al. [95]            | 2020 |     | 1    |          |          | [6,10]  |                            | Human-Machine Interaction |
| Setiawan et al. [96]         | 2020 |     | 1    | 1        |          | [0,5]   |                            | Human-Machine Interaction |
| Jiang et al. [97]            | 2020 |     | 1    |          |          | [6,10]  |                            | Human-Machine Interaction |
| Nassour et al. [98]          | 2020 |     | 1    |          |          | [11,18] |                            | Human-Machine Interaction |
| Vu et al. [99]               | 2020 |     |      | 1        |          |         | 1,00                       | None                      |
| Zhang et al. [100]           | 2020 |     | 1    |          |          | [6,10]  |                            | None                      |
| Chauhan et al. [101]         | 2020 |     | 1    |          |          | [0,5]   |                            | Environment Interaction   |
| Chitra et al. [102]          | 2020 | 1   | 1    |          |          | [6,10]  |                            | Human-Machine Interaction |
| Pan et al. [103]             | 2020 |     |      | 1        |          |         | 12,56                      | Human-Machine Interaction |
| Sabry et al. [104]           | 2020 |     | 1    | 1        |          | [0,5]   | 3,93                       | Functionality Assessment  |
| Hazman et al. [105]          | 2020 | 1   | 1    |          |          | [0,5]   |                            | Environment Interaction   |
| Jhamb et al. [106]           | 2020 | 1   | 1    |          |          | [6,10]  |                            | Human-Machine Interaction |
| Kim et al. [107]             | 2020 |     | 1    |          |          | [0,5]   |                            | Functionality Assessment  |
| Noh et al. [108]             | 2020 |     | 1    |          |          | [0,5]   |                            | Human-Machine Interaction |
| Steffen et al. [109]         | 2020 |     |      | 1        |          |         | 0,50                       | Environment Interaction   |
| Ayodele et al. [110]         | 2021 |     | 1    |          |          | [0,5]   |                            | Environment Interaction   |
| Ayodele et al. [111]         | 2021 |     | 1    |          |          | [0,5]   |                            | Environment Interaction   |
| Zhang et al. [112]           | 2021 |     | 1    |          |          | [6,10]  |                            | Human-Machine Interaction |
| Tsai et al. [113]            | 2021 | 1   | 1    | 1        |          | [6,10]  |                            | Human-Machine Interaction |
| Ahmed et al. [114]           | 2021 | 1   | 1    | 1        |          | [11,18] | 10,49                      | Human-Machine Interaction |
| Fei et al. [115]             | 2021 | 1   |      |          |          | [19+]   |                            | Functionality Assessment  |
| Lee et al. [116]             | 2021 |     | 1    |          |          | [6,10]  |                            | Human-Machine Interaction |
| Li et al. [117]              | 2021 | 1   | 1    |          |          | [6,10]  |                            | None                      |
| Li et al. [118]              | 2021 |     | 1    |          |          | [6,10]  |                            | Human-Machine Interaction |

TABLE I: The table contains the results of the classification described in this publication - continued.

| Author                   | Year | IMU | Flex | Pressure | Magnetic | DoFs    | P. Area (cm <sup>2</sup> ) | Application               |
|--------------------------|------|-----|------|----------|----------|---------|----------------------------|---------------------------|
| Muezzinoglu et al. [119] | 2021 | 1   | 1    |          |          | [6,10]  |                            | Human-Machine Interaction |
| Santoni et al. [120]     | 2021 |     |      |          | 1        | [11,18] |                            | Environment Interaction   |
| Shin et al. [121]        | 2021 |     | 1    |          |          | [6,10]  |                            | Human-Machine Interaction |
| Wang et al. [122]        | 2021 |     |      | 1        |          |         | 7,20                       | Environment Interaction   |
| Yuan et al. [123]        | 2021 | 1   | 1    |          |          | [11,18] |                            | Human-Machine Interaction |
| Yuan et al. [124]        | 2021 |     | 1    |          |          | [0,5]   |                            | Human-Machine Interaction |
| Simoes Dias et al. [125] | 2022 | 1   | 1    | 1        |          | [6,10]  | 9,33                       | Human-Machine Interaction |
| Dutta et al. [126]       | 2022 | 1   | 1    |          |          | [6,10]  |                            | Functionality Assessment  |
| Lee et al. [127]         | 2022 |     | 1    |          |          | [6,10]  |                            | Human-Machine Interaction |
| Li et al. [128]          | 2021 | 1   |      |          |          | [19+]   |                            | Environment Interaction   |
| Sarwat et al. [129]      | 2021 | 1   | 1    | 1        |          | [11,18] | 2,28                       | Functionality Assessment  |
| Choi et al. [130]        | 2021 |     |      | 1        |          |         |                            | Environment Interaction   |
| Fu et al. [131]          | 2021 | 1   | 1    |          |          | [6,10]  |                            | Human-Machine Interaction |
| Cazacu et al. [132]      | 2021 |     |      |          | 1        |         |                            | Functionality Assessment  |
| Alrubayi et al. [133]    | 2021 | 1   | 1    | 1        |          | [11,18] | 10,49                      | Human-Machine Interaction |
| Biju et al. [134]        | 2021 |     | 1    | 1        |          | [0,5]   | 13,68                      | Environment Interaction   |
| Ahmed et al. [135]       | 2021 | 1   | 1    | 1        |          | [11,18] | 10,49                      | Human-Machine Interaction |
| Wu et al. [136]          | 2021 |     | 1    |          |          | [11,18] |                            | Human-Machine Interaction |
| Maitre et al. [137]      | 2021 |     | 1    | 1        |          | [6,10]  | 3,56                       | Environment Interaction   |
| Sim et al. [138]         | 2021 |     | 1    |          |          | [6,10]  |                            | Human-Machine Interaction |
| Guo et al. [139]         | 2021 |     | 1    |          |          | [0,5]   |                            | Human-Machine Interaction |
| Gosala et al. [140]      | 2021 | 1   | 1    |          |          | [19+]   |                            | Human-Machine Interaction |
| Davarzani et al. [141]   | 2021 | 1   |      |          |          | [0,5]   |                            | Functionality Assessment  |
| Han et al. [142]         | 2021 |     | 1    |          |          | [0,5]   |                            | Human-Machine Interaction |
| Calado et al. [143]      | 2021 | 1   | 1    |          |          | [11,18] |                            | Human-Machine Interaction |
| Dong et al. [144]        | 2021 | 1   | 1    |          |          | [6,10]  |                            | Human-Machine Interaction |
| Aw et al. [145]          | 2022 |     | 1    |          |          | [6,10]  |                            | Human-Machine Interaction |
| Hwang et al. [146]       | 2022 | 1   |      |          |          | [19+]   |                            | Functionality Assessment  |
| Elwahsh et al. [147]     | 2022 | 1   | 1    |          |          | [6,10]  |                            | Human-Machine Interaction |
| Antillon et al. [148]    | 2022 | 1   | 1    |          |          | [6,10]  |                            | Human-Machine Interaction |
| Wang et al. [149]        | 2022 | 1   |      |          |          | [6,10]  |                            | Human-Machine Interaction |
| Boruah et al. [150]      | 2022 |     | 1    |          |          | [0,5]   |                            | Environment Interaction   |
| Yudhana et al. [151]     | 2022 |     | 1    |          |          | [0,5]   |                            | Human-Machine Interaction |
| Zhang et al. [152]       | 2022 |     | 1    |          |          | [0,5]   |                            | Human-Machine Interaction |
| Duan et al. [153]        | 2022 |     | 1    |          |          | [0,5]   |                            | Human-Machine Interaction |
| Huang et al. [154]       | 2022 |     | 1    |          |          | [0,5]   |                            | Human-Machine Interaction |
| Maddahi et al. [155]     | 2022 | 1   | 1    |          |          | [6,10]  |                            | Functionality Assessment  |
| Bright et al. [156]      | 2022 | 1   |      |          |          | [19+]   |                            | Human-Machine Interaction |
| Kerner et al. [157]      | 2022 | 1   |      | 1        |          | [0,5]   | 0,79                       | Environment Interaction   |
| Zhou et al. [158]        | 2022 | 1   |      |          |          | [11,18] |                            | Human-Machine Interaction |
| Zheng et al. [159]       | 2022 | 1   | 1    | 1        |          | [6,10]  | 11,78                      | Environment Interaction   |
| Anbalagan et al. [160]   | 2022 | 1   |      |          |          | [0,5]   |                            | Functionality Assessment  |
| Elkasass et al. [161]    | 2022 |     | 1    |          |          | [0,5]   |                            | Human-Machine Interaction |
| Piskozub et al. [162]    | 2022 |     | 1    |          |          | [6,10]  |                            | Human-Machine Interaction |
| Lin et al. [163]         | 2022 | 1   | 1    |          |          | [0,5]   |                            | Human-Machine Interaction |
| Calado et al. [164]      | 2022 | 1   | 1    |          |          | [6,10]  |                            | Human-Machine Interaction |
| Biju et al. [165]        | 2022 |     | 1    | 1        |          | [0,5]   |                            | Environment Interaction   |
| DelPreto et al. [166]    | 2022 | 1   | 1    |          |          | [11,18] |                            | Human-Machine Interaction |
| Zhang et al. [167]       | 2022 |     | 1    |          |          | [6,10]  |                            | Human-Machine Interaction |
| Lin et al. [168]         | 2022 | 1   |      |          |          | [19+]   |                            | Functionality Assessment  |
| Cerqueira et al. [169]   | 2022 | 1   |      |          |          | [19+]   |                            | Environment Interaction   |
| Hekmat et al. [170]      | 2022 |     | 1    |          |          | [0,5]   |                            | Human-Machine Interaction |
| Sadhu et al. [171]       | 2022 | 1   | 1    |          |          | [6,10]  |                            | Functionality Assessment  |
| Zakri et al. [172]       | 2022 |     | 1    |          |          | [0,5]   |                            | Human-Machine Interaction |
| Yu et al. [173]          | 2022 | 1   | 1    |          |          | [6,10]  |                            | Human-Machine Interaction |
| Liao et al. [174]        | 2022 |     |      | 1        |          |         |                            | Environment Interaction   |
| Huang et al. [175]       | 2022 | 1   |      |          |          | [11,18] |                            | Human-Machine Interaction |
| Luo et al. [176]         | 2023 |     | 1    |          |          | [0,5]   |                            | Human-Machine Interaction |
| Simoes Dias et al. [177] | 2023 | 1   | 1    |          |          | [6,10]  |                            | Human-Machine Interaction |

## REFERENCES

- [1] D. T. Rand and A. C. Nicol, "An instrumented glove for monitoring mcp joint motion," *Proceedings of the Institution of Mechanical Engineers, Part H: Journal of Engineering in Medicine*, vol. 207, no. 4, pp. 207–210, 1993.
- [2] N. Karlsson, B. Karlsson, and P. Wide, "A glove equipped with finger flexion sensors as a command generator used in a fuzzy control system," *IEEE Transactions on Instrumentation and Measurement*, vol. 47, no. 5, pp. 1330–1334, 1998.
- [3] S. Crook and P. Chappell, "A portable system for closed loop control of the paralysed hand using functional electrical stimulation," *Medical Engineering & Physics*, vol. 20, no. 1, pp. 70–76, 1998.
- [4] S. You, T. Wang, R. Eagleson, C. Meng, and Q. Zhang, "A low-cost internet-based telerobotic system for access to remote laboratories," *Artif. Intell. Eng.*, vol. 15, pp. 265–279, 2001.
- [5] M. Bouzit, G. Burdea, G. Popescu, and R. Boian, "The rutgers master ii-new design force-feedback glove," *IEEE/ASME Transactions on Mechatronics*, vol. 7, no. 2, pp. 256–263, 2002.
- [6] A. Mazzoldi, D. D. Rossi, F. Lorussi, E. P. Scilingo, and R. Paradiso, "Smart textiles for wearable motion capture systems," *AUTEX Research Journal*, vol. 2, no. 4, pp. 199–203, 2002.
- [7] K. Tarchanidis and J. Lygouras, "Data glove with a force sensor," *IEEE T. Instrumentation and Measurement*, vol. 52, no. 3, pp. 984–989, 2003.
- [8] Y. Su, C. Allen, D. Geng, D. Burn, U. Brechany, G. Bell, and R. Rowland, "3-d motion system ("data-gloves"): application for parkinson's disease," *IEEE Transactions on Instrumentation and Measurement*, vol. 52, no. 3, pp. 662–674, 2003.
- [9] J. Ku, R. Mraz, N. Baker, K. K. Zakzanis, J.-H. Lee, I.-Y. Kim, S. I. Kim, and S. J. Graham, "A data glove with tactile feedback for fmri of virtual reality experiments," *Cyberpsychology & behavior : the impact of the Internet, multimedia and virtual reality on behavior and society*, vol. 6 5, pp. 497–508, 2003.
- [10] R. Mraz, J. Hong, G. Quintin, W. R. Staines, W. E. McIlroy, K. K. Zakzanis, and S. J. Graham, "A platform for combining virtual reality experiments with functional magnetic resonance imaging," *CyberPsychology & Behavior*, vol. 6, no. 4, pp. 359–368, 2003.
- [11] C.-S. Fahn and H. Sun, "Development of a data glove with reducing sensors based on magnetic induction," *IEEE Transactions on Industrial Electronics*, vol. 52, no. 2, pp. 585–594, 2005.
- [12] G. Bao, "Force feedback dataglove based on pneumatic artificial muscles," *Chinese Journal of Mechanical Engineering - CHIN J MECH ENG*, vol. 19, no. 4, p. 588, 2006.
- [13] T. D. Bui and L. Thang Nguyen, "Recognizing postures in vietnamese sign language with mems accelerometers," *IEEE Sensors Journal*, vol. 7, no. 5, pp. 707–712, 2007.
- [14] Y. Su, M. Fisher, A. Wolczowski, G. Bell, D. Burn, and R. Gao, "Towards an emg controlled prosthetic hand using a 3d electromagnetic positioning system," in *IEEE Instrumentation and Measurement Technology Conference Proceedings*, Ottawa, ON, Canada, May 2005.
- [15] E. Komi, J. Roberts, and S. Rothberg, "Measurement and analysis of grip force during a golf shot," *Proceedings of the Institution of Mechanical Engineers Part P Journal of Sports Engineering and Technology*, vol. 222, pp. 23–35, 2008.
- [16] F. Amirouche, J. R. Martin, M. Gonzalez, and L. Fergusson, "Experimental set-up and sensory glove interface for microsurgery," *Proceedings of the Institution of Mechanical Engineers, Part H: Journal of Engineering in Medicine*, vol. 222, no. 1, pp. 89–99, 2008.
- [17] R. C. King, L. Atallah, B. P. L. Lo, and G.-Z. Yang, "Development of a wireless sensor glove for surgical skills assessment," *IEEE Transactions on Information Technology in Biomedicine*, vol. 13, no. 5, pp. 673–679, 2009.
- [18] L. Maréchal, C. Barthod, and J.-C. Jeulin, "First characterization of the expiratory flow increase technique: method development and results analysis," *Physiological measurement*, vol. 30, no. 12, p. 1445, 2009.
- [19] Y.-F. Fu and C.-S. Ho, "A user-dependent easily-adjusted static finger language recognition system for handicapped aphasiacs," *Applied Artificial Intelligence*, vol. 23, no. 10, pp. 932–944, 2009.
- [20] C.-S. Fahn and H. Sun, "Development of a fingertip glove equipped with magnetic tracking sensors," *Sensors (Basel, Switzerland)*, vol. 10, no. 2, pp. 1119–40, 2010.
- [21] L. Gallo, *A Glove-Based Interface for 3D Medical Image Visualization*. Springer, 2010, pp. 221–230.
- [22] Y.-F. Fu and C.-S. Ho, "Building intelligent communication systems for handicapped aphasiacs," *Sensors*, vol. 10, no. 1, pp. 374–387, 2010.
- [23] H. Wang, M. Jeon, and Y.-G. Lee, "New design of a virtualglove for grasping applications," *Human Factors in Ergonomics & Manufacturing*, vol. 20, no. 4, pp. 353–364, 2010.
- [24] A. F. Da Silva, A. F. Gonçalves, P. M. Mendes, and J. H. Correia, "Fbg sensing glove for monitoring hand posture," *IEEE Sensors Journal*, vol. 11, no. 10, pp. 2442–2448, 2011.
- [25] S. Dalley, A. Varol, and M. Goldfarb, "A method for the control of multigrasp myoelectric prosthetic hands," *IEEE transactions on neural systems and rehabilitation engineering : a publication of the IEEE Engineering in Medicine and Biology Society*, vol. 20, no. 1, pp. 58–67, 2011.
- [26] P. Falco, G. De Maria, C. Natale, and S. Pirozzi, "Data fusion based on optical technology for observation of human manipulation," *International Journal of Optomechatronics*, vol. 6, no. 1, pp. 37–70, 2012.
- [27] E. Fujiwara, Y. T. Wu, D. Y. Miyatake, M. F. Santos, and C. K. Suzuki, "Evaluation of thumb-operated directional pad functionalities on a glove-based optical fiber sensor," *IEEE Transactions on Instrumentation and Measurement*, vol. 62, no. 8, pp. 2330–2337, 2013.
- [28] N. Tongrod, S. Lokavee, N. Wathanawisuth, and A. Tuantranont, "Design and development of data glove based on printed polymeric sensors and zigbee networks for human-computer interface," *Disability and rehabilitation. Assistive technology*, vol. 8, no. 2, pp. 115–20, 2013.
- [29] E. Fujiwara, M. Santos, and C. Suzuki, "Flexible optical fiber bending transducer for application in glove-based sensors," *Sensors Journal, IEEE*, vol. 14, pp. 3631–3636, 10 2014.
- [30] A. C. Yuen, A. A. Bakir, N. N. Z. M. Rajdi, C. L. Lam, S. M. Saleh, and D. H. Wicaksono, "Proprioceptive sensing system for therapy assessment using cotton fabric-based biomedical microelectromechanical system," *IEEE Sensors Journal*, vol. 14, no. 8, pp. 2872–2880, 2014.
- [31] E. Tanaka, S. Saegusa, Y. Iwasaki, and L. Yuge, "Development of an adl assistance apparatus for upper limbs and evaluation of muscle and cerebral activity of the user," *Journal of Advanced Mechanical Design Systems and Manufacturing*, vol. 8, 2013.
- [32] A. Z. Shukor, M. F. Miskon, M. H. Jamaluddin, F. bin Ali, M. F. Asyraf, M. B. bin Bahar *et al.*, "A new data glove approach for malaysian sign language detection," *Procedia Computer Science*, vol. 76, pp. 60–67, 2015.
- [33] C. Schuster-Amft, A. Henneke, B. Hartog-Keisker, L. Holper, E. Siekierka, E. Chevrier, P. Pyk, S. Kollias, D. Kiper, and K. Eng, "Intensive virtual reality-based training for upper limb motor function in chronic stroke: A feasibility study using a single case experimental design and fmri," *Disability and rehabilitation. Assistive technology*, vol. 10, no. 5, pp. 385–392, 2014.
- [34] K.-W. Kim, M.-S. Lee, B.-R. Soon, M.-H. Ryu, and J.-N. Kim, "Recognition of sign language with an inertial sensor-based data glove," *Technology and Health Care*, vol. 24, no. s1, pp. S223–S230, 2016.
- [35] P.-J. Chen and Y.-C. Du, "Combining independent component and grey relational analysis for the real-time system of hand motion identification using bend sensors and multichannel surface emg," *Mathematical Problems in Engineering*, vol. 2015, pp. 1–9, 2015.
- [36] P. Girovský and M. Kunderát, "Robotic arm based dynamixel actuators controlled by the data glove," *International Journal of Engineering Research in Africa*, vol. 18, p. 152–158, 2015.
- [37] G. K. Saini and R. Kaur, "Designing real-time virtual instrumentation system for differently abled using labview," *International Journal of Biomedical Engineering and Technology*, vol. 18, no. 1, pp. 86–101, 2015.
- [38] J. Galka, M. Masior, M. Zaborski, and K. Barczewska, "Inertial motion sensing glove for sign language gesture acquisition and recognition," *IEEE Sensors Journal*, vol. 16, no. 16, pp. 6310–6316, 2016.

- [39] K. Li, Z. Zhou, and C.-H. Lee, "Sign transition modeling and a scalable solution to continuous sign language recognition for real-world applications," *ACM Transactions on Accessible Computing (TACCESS)*, vol. 8, no. 2, pp. 1–23, 2016.
- [40] F. Lorussi, N. Carbonaro, D. De Rossi, R. Paradiso, P. Veltink, and A. Tognetti, "Wearable textile platform for assessing stroke patient treatment in daily life conditions," *Frontiers in bioengineering and biotechnology*, vol. 4, p. 28, 2016.
- [41] J. Liu, Y. Luo, and Z. Ju, "An interactive astronaut-robot system with gesture control," *Computational intelligence and neuroscience*, vol. 2016, 2016.
- [42] D. H. Kim, S. W. Lee, and H.-S. Park, "Improving kinematic accuracy of soft wearable data gloves by optimizing sensor locations," *Sensors*, vol. 16, no. 6, p. 766, 2016.
- [43] R. Tavares, P. Abreu, and M. R. Quintas, "Data acquisition glove for hand movement impairment rehabilitation," *Int. J. Online Eng.*, vol. 12, no. 4, pp. 52–54, 2016.
- [44] A. I. Che-Ani, A. Othman, N. Hamzah, A. D. Rosli, R. Baharudin, and M. F. Abdullah, "Real-time finger hand movement capturing via a data hand glove," *ARPN journal of engineering and applied sciences*, vol. 11, pp. 4877–4881, 2016.
- [45] N. E. H. Saleh, A. Hage-Diab, G. Salhab, B. Debs, M. Hajj-Hassan, H. Khachfe, A. R. Sarraj, and S. Saleh, "Monitoring the use of impaired hand by a new low cost device during daily life activities with real-time visual feedback," *International Journal on Advances in Life Sciences*, vol. 8, no. 1&2, 2016.
- [46] M. Yahya, N. Hamzah, A. Othman, A. Diyana, R. Baharudin, and A. I. Che Ani, "Design and development of a mirror effect control prosthetic hand with force sensing," *Telkomnika (Telecommunication Computing Electronics and Control)*, vol. 15, no. 2, pp. 949–956, 2017.
- [47] B.-S. Lin, P.-C. Hsiao, S.-Y. Yang, C.-S. Su, and I.-J. Lee, "Data glove system embedded with inertial measurement units for hand function evaluation in stroke patients," *IEEE Transactions on Neural Systems and Rehabilitation Engineering*, vol. 25, no. 11, pp. 2204–2213, 2017.
- [48] A. S. Zuruzi, T. M. Haffiz, D. Affidah, A. Amirul, A. Norfatriah, and M. H. Nurmawati, "Towards wearable pressure sensors using multiwall carbon nanotube/polydimethylsiloxane nanocomposite foams," *Materials & Design*, vol. 132, pp. 449–458, 2017.
- [49] B. Fang, F. Sun, H. Liu, and D. Guo, "A novel data glove using inertial and magnetic sensors for motion capture and robotic arm-hand teleoperation," *Industrial Robot: An International Journal*, vol. 44, pp. 155–165, 2017.
- [50] Y. Lin, J. Breugelmans, M. Iversen, and D. Schmidt, "An adaptive interface design (aid) for enhanced computer accessibility and rehabilitation," *International Journal of Human-Computer Studies*, vol. 98, 2016.
- [51] A. Asadipour, K. Debatista, and A. Chalmers, "Visuohaptic augmented feedback for enhancing motor skills acquisition," *The Visual Computer*, vol. 33, no. 4, pp. 401–411, 2017.
- [52] Y. Ganjdanesh, K. Maghooli, A. M. Nasrabadi, and M.-S. Moein, "A new method for signature verification based on physiological characteristics of hand muscles and tendons," *Biomedical Engineering: Applications, Basis and Communications*, vol. 29, no. 01, p. 1750006, 2017.
- [53] J. Connolly, J. Condell, B. O'Flynn, J. T. Sanchez, and P. Gardiner, "Imu sensor-based electronic goniometric glove for clinical finger movement analysis," *IEEE Sensors Journal*, vol. 18, no. 3, pp. 1273–1281, 2018.
- [54] B.-S. Lin, I.-J. Lee, S.-Y. Yang, Y.-C. Lo, J. Lee, and J.-L. Chen, "Design of an inertial-sensor-based data glove for hand function evaluation," *Sensors*, vol. 18, no. 5, p. 1545, 2018.
- [55] C. K. Mummadi, F. P. P. Leo, K. D. Verma, S. Kasireddy, P. M. Scholl, J. Kempfle, and K. V. Laerhoven, "Real-time and embedded detection of hand gestures with an imu-based glove," *Informatics*, vol. 5, no. 2, 2018.
- [56] X. Liao, W. Wang, M. Lin, M. Li, H. Wu, and Y. Zheng, "Hierarchically distributed microstructure design of haptic sensors for personalized fingertip mechanosensational manipulation," *Materials Horizons*, vol. 5, no. 5, pp. 920–931, 2018.
- [57] C. Lu, J. Chen, T. Jiang, G. Gu, W. Tang, and Z. L. Wang, "A stretchable, flexible triboelectric nanogenerator for self-powered real-time motion monitoring," *Advanced Materials Technologies*, vol. 3, no. 6, p. 1800021, 2018.
- [58] Y. Choi, K. Yoo, S. J. Kang, B. Seo, and S. K. Kim, "Development of a low-cost wearable sensing glove with multiple inertial sensors and a light and fast orientation estimation algorithm," *The Journal of Supercomputing*, vol. 74, no. 8, pp. 3639–3652, 2018.
- [59] T. Kanokoda, Y. Kushitani, M. Shimada, and J.-i. Shirakashi, "Gesture prediction using wearable sensing systems with neural networks for temporal data analysis," *Sensors*, vol. 19, no. 3, p. 710, 2019.
- [60] G. Saldaña González, J. Cerezo Sánchez, M. M. Bustillo Díaz, and A. Ata Pérez, "Recognition and classification of sign language for spanish," *Computación y Sistemas*, vol. 22, no. 1, pp. 271–277, 2018.
- [61] S. Shahrapour, M. Noshad, J. Ding, and V. Tarokh, "Online learning for multimodal data fusion with application to object recognition," *IEEE Transactions on Circuits and Systems II: Express Briefs*, vol. 65, no. 9, pp. 1259–1263, 2017.
- [62] M. Hoda, Y. Hoda, B. Hafidh, and A. El Saddik, "Predicting muscle forces measurements from kinematics data using kinect in stroke rehabilitation," *Multimedia Tools and Applications*, vol. 77, no. 2, pp. 1885–1903, 2018.
- [63] C.-H. Kao, C.-C. Chen, W.-Y. Jhu, Y.-T. Tsai, S.-H. Chen, C.-M. Hsu, and C.-Y. Chen, "Novel digital glove design for virtual reality applications," *Microsystem Technologies*, vol. 24, no. 10, pp. 4247–4266, 2018.
- [64] F. Malawski and J. Galka, "System for multimodal data acquisition for human action recognition," *Multimedia Tools and Applications*, vol. 77, no. 18, pp. 23 825–23 850, 2018.
- [65] Y. F. Chacon, M. Plaza, and A. M. Cifuentes, "Development and design wearable sensorial system of low cost to determine the metacarpophalangeal and interphalangeal joints angles," *ECS Transactions*, vol. 86, no. 16, p. 39, 2018.
- [66] M. Javaid, "Communication through haptics during human collaborative manipulation," *International Journal of Humanoid Robotics*, vol. 15, no. 03, p. 1850003, 2018.
- [67] O. Glauser, S. Wu, D. Panozzo, O. Hilliges, and O. Sorkine-Hornung, "Interactive hand pose estimation using a stretch-sensing soft glove," *ACM Transactions on Graphics (TOG)*, vol. 38, no. 4, pp. 1–15, 2019.
- [68] Q. Zhang, Y. L. Wang, Y. Xia, P. F. Zhang, T. V. Kirk, and X. D. Chen, "Textile-only capacitive sensors for facile fabric integration without compromise of wearability," *Advanced Materials Technologies*, vol. 4, no. 10, p. 1900485, 2019.
- [69] X. Zhang, Z. Yang, T. Chen, D. Chen, and M.-C. Huang, "Cooperative sensing and wearable computing for sequential hand gesture recognition," *IEEE Sensors Journal*, vol. 19, no. 14, pp. 5775–5783, 2019.
- [70] X. Huang, Q. Wang, S. Zang, J. Wan, G. Yang, Y. Huang, and X. Ren, "Tracing the motion of finger joints for gesture recognition via sewing rgo-coated fibers onto a textile glove," *IEEE sensors journal*, vol. 19, no. 20, pp. 9504–9511, 2019.
- [71] B.-S. Lin, I.-J. Lee, P.-Y. Chiang, S.-Y. Huang, and C.-W. Peng, "A modular data glove system for finger and hand motion capture based on inertial sensors," *Journal of Medical and Biological Engineering*, vol. 39, 06 2018.
- [72] V. Stornelli, A. Leoni, G. Ferri, V. Errico, A. Pallotti, G. Orengo, and G. Saggio, "A 10-17 dof sensory gloves with harvesting capability for smart healthcare," *Journal of Communications Software and Systems*, vol. 15, no. 2, pp. 166–172, 2019.
- [73] H. Kim and Y. Choi, "Performance comparison of user interface devices for controlling mining software in virtual reality environments," *Applied Sciences*, vol. 9, no. 13, p. 2584, 2019.
- [74] B.-S. Lin, I.-J. Lee, P.-C. Hsiao, and Y.-T. Hwang, "An assessment system for post-stroke manual dexterity using principal component analysis and logistic regression," *IEEE Transactions on Neural Systems and Rehabilitation Engineering*, vol. 27, no. 8, pp. 1626–1634, 2019.
- [75] V. Mehra, A. Choudhury, and R. R. Choubey, "Gesture to speech conversion using flex sensors mpu6050 and python," *Published in International Journal of Engineering and Advanced Technology (IJEAT)*, vol. 8, no. 6, pp. 4686–4690, 2019.
- [76] W.-C. Chuang, W.-J. Hwang, T.-M. Tai, D.-R. Huang, and Y.-J. Jhang, "Continuous finger gesture recognition based on flex sensors," *Sensors*, vol. 19, no. 18, p. 3986, 2019.

- [77] L. Jiang, H. Xia, and C. Guo, "A model-based system for real-time articulated hand tracking using a simple data glove and a depth camera," *Sensors*, vol. 19, no. 21, p. 4680, 2019.
- [78] S. Li, R. Rameshwar, A. M. Votta, and C. D. Onal, "Intuitive control of a robotic arm and hand system with pneumatic haptic feedback," *IEEE Robotics and Automation Letters*, vol. 4, no. 4, pp. 4424–4430, 2019.
- [79] Q. Liu, G. Qian, W. Meng, Q. Ai, C. Yin, and Z. Fang, "A new immu-based data glove for hand motion capture with optimized sensor layout," *International Journal of Intelligent Robotics and Applications*, vol. 3, no. 1, pp. 19–32, 2019.
- [80] A. Melynyk and P. Hénaff, "Physical analysis of handshaking between humans: mutual synchronisation and social context," *International Journal of Social Robotics*, vol. 11, no. 4, pp. 541–554, 2019.
- [81] V. Minh, N. Katushin, and J. Pumwa, "Motion tracking glove for augmented reality and virtual reality," *Paladyn, Journal of Behavioral Robotics*, vol. 10, no. 1, pp. 160–166, 2019.
- [82] S. Ullah, Z. Mumtaz, S. Liu, M. Abubaqr, A. Mahboob, and H. A. Madni, "Single-equipment with multiple-application for an automated robot-car control system," *Sensors*, vol. 19, no. 3, p. 662, 2019.
- [83] Y. Yao, S. Rakheja, and P. Marcotte, "Relationship among hand forces imparted on a viscoelastic hand-handle interface," *Measurement*, vol. 145, pp. 525–534, 2019.
- [84] R. Z. R. Umar, C. F. Ling, N. Abdullasim, N. Ahmad, I. Halim, and M. Hamid, "Occupational wrist postural assessment and monitoring system: development and initial validation," *Journal of Engineering Science and Technology*, vol. 14, no. 6, pp. 3421–3426, 2019.
- [85] W. Zhang, J. Z. Yu, F. Zhu, Y. Zhu, Z. Yang, N. G. Ulu, B. Arisoy, and L. B. Kara, "High degree of freedom hand pose tracking using limited strain sensing and optical training," *Journal of Computing and Information Science in Engineering*, vol. 19, no. 3, 2019.
- [86] C. Lim, H. sang Ko, S. Cho, I. Ohu, H. E. Wang, B. Jimmy, J. Felice, R. E. Griffin, and J. N. Carlson, "Development of classification models for assessment of endotracheal intubation training by a cyber-physical system," *Procedia Manufacturing*, vol. 39, pp. 357–362, 2019.
- [87] G. Puasa, "Data glove for american sign language alphabet and numbers (1-9) translation system," *International Journal of Advanced Trends in Computer Science and Engineering*, vol. 8, no. 4, pp. 1128–1133, 2019.
- [88] V. Shweta, D. A. Asarpota, H. Verma *et al.*, "User trainable sign language to speech glove using knn classifier," *Compusoft*, vol. 3053, no. 3058, p. 8, 2019.
- [89] S. A. A. Syed Mubarak Ali, N. S. Ahmad, and P. Goh, "Flex sensor compensator via hammerstein–wiener modeling approach for improved dynamic goniometry and constrained control of a bionic hand," *Sensors*, vol. 19, no. 18, p. 3896, 2019.
- [90] M. Abtahi, S. B. Borgheai, R. Jafari, N. Constant, R. Diouf, Y. Shahriari, and K. Mankodiya, "Merging fnirs-eeg brain monitoring and body motion capture to distinguish parkinsons disease," *IEEE Transactions on Neural Systems and Rehabilitation Engineering*, vol. 28, no. 6, pp. 1246–1253, 2020.
- [91] J. Song, S. Chen, L. Sun, Y. Guo, L. Zhang, S. Wang, H. Xuan, Q. Guan, and Z. You, "Mechanically and electronically robust transparent organohydrogel fibers," *Advanced Materials*, vol. 32, no. 8, p. 1906994, 2020.
- [92] L. Zhang, J. Pan, Z. Zhang, H. Wu, N. Yao, D. Cai, Y. Xu, J. Zhang, G. Sun, L. Wang *et al.*, "Ultrasensitive skin-like wearable optical sensors based on glass micro/nanofibers," *Opto-Electronic Advances*, vol. 3, no. 3, pp. 190 022–1, 2020.
- [93] H.-T. Chang and J.-Y. Chang, "Sensor glove based on novel inertial sensor fusion control algorithm for 3-d real-time hand gestures measurements," *IEEE Transactions on Industrial Electronics*, vol. 67, no. 1, pp. 658–666, 2020.
- [94] C.-Z. Hang, X.-F. Zhao, S.-Y. Xi, Y.-H. Shang, K.-P. Yuan, F. Yang, Q.-G. Wang, J.-C. Wang, D. W. Zhang, and H.-L. Lu, "Highly stretchable and self-healing strain sensors for motion detection in wireless human-machine interface," *Nano Energy*, vol. 76, p. 105064, 2020.
- [95] Y. Zhang, Y. Huang, X. Sun, Y. Zhao, X. Guo, P. Liu, C. Liu, and Y. Zhang, "Static and dynamic human arm/hand gesture capturing and recognition via multiinformation fusion of flexible strain sensors," *IEEE Sensors Journal*, vol. 20, no. 12, pp. 6450–6459, 2020.
- [96] J. D. Setiawan, M. Ariyanto, M. Munadi, M. Mutoha, A. Glowacz, and W. Caesarendra, "Grasp posture control of wearable extra robotic fingers with flex sensors based on neural network," *Electronics*, vol. 9, no. 6, p. 905, 2020.
- [97] Y. Jiang, V. Reimer, T. Schossig, M. Angelmahr, and W. Schade, "Fiber optical multifunctional human-machine interface for motion capture, temperature, and contact force monitoring," *Optics and Lasers in Engineering*, vol. 128, p. 106018, 2020.
- [98] J. Nassour, H. G. Amirabadi, S. Weheabby, A. Al Ali, H. Lang, and F. Hamker, "A robust data-driven soft sensory glove for human hand motions identification and replication," *IEEE Sensors Journal*, vol. 20, no. 21, pp. 12972–12979, 2020.
- [99] C. C. Vu and J. Kim, "Highly elastic capacitive pressure sensor based on smart textiles for full-range human motion monitoring," *Sensors and Actuators A: Physical*, vol. 314, p. 112029, 2020.
- [100] Y. Zhang, Y. Huang, P. Liu, C. Liu, X. Guo, and Y. Zhang, "Highly stretchable strain sensor with wide linear region via hydrogen bond-assisted dual-mode cooperative conductive network for gait detection," *Composites Science and Technology*, vol. 191, p. 108070, 2020.
- [101] R. Chauhan, B. Sebastian, and P. Ben-Tzvi, "Grasp prediction toward naturalistic exoskeleton glove control," *IEEE transactions on human-machine systems*, vol. 50, no. 1, pp. 22–31, 2019.
- [102] P. Chitra, S. Manickam, R. Prabha, A. Sahaya, A. Nisha, and T. Bernatin, "Gloves gesture recognition," *International Journal of Scientific & Technology Research*, 05 2022.
- [103] J. Pan, Y. Luo, Y. Li, C.-K. Tham, C.-H. Heng, and A. V.-Y. Thean, "A wireless multi-channel capacitive sensor system for efficient glove-based gesture recognition with ai at the edge," *IEEE Transactions on Circuits and Systems II: Express Briefs*, vol. 67, no. 9, pp. 1624–1628, 2020.
- [104] S. Sabry, M. Sahib, and T. Nayl, "Toward hand functions rehabilitation using the virtual world for pre-school children with cerebral palsy," *International Journal of Emerging Technologies in Learning (iJET)*, vol. 15, no. 9, pp. 110–122, 2020.
- [105] M. Hazman, I. N. A. Mohd Nordin, F. Hanim, N. Khamis, M. Razif, A. A. Mohd Faudzi, and A. Mohd Hanif, "Imu sensor-based data glove for finger joint measurement," *Indonesian Journal of Electrical Engineering and Computer Science*, vol. 20, no. 1, pp. 82–88, 2020.
- [106] P. Jhamb and A. Rehalia, "Wireless hand gesture controlled multiple musical instruments," *International Journal of Information Technology*, vol. 12, no. 1, pp. 19–25, 2020.
- [107] J. Kim, G. Lee, H. Jo, W. Park, Y. S. Jin, H. D. Kim, and J. Kim, "A wearable soft robot for stroke patients' finger occupational therapy and quantitative measures on the joint paralysis," *International Journal of Precision Engineering and Manufacturing*, vol. 21, no. 12, pp. 2419–2426, 2020.
- [108] J. S. Noh, S. K. Lee, and Y. Y. Kim, "Development of hand motion tracking device for agricultural machinery simulator," *Journal of Biosystems Engineering*, vol. 45, no. 4, pp. 401–408, 2020.
- [109] B. Steffen, G. Christian, B. Rainer, N. Nina, M. Wolfram, and S. Katrin, "Wearable pressure sensing for vojta therapy guidance," *Current Directions in Biomedical Engineering*, vol. 6, no. 3, pp. 87–90, 2020.
- [110] E. Ayodele, T. Bao, S. A. R. Zaidi, A. M. Hayajneh, J. Scott, Z.-Q. Zhang, and D. McLernon, "Grasp classification with weft knit data glove using a convolutional neural network," *IEEE Sensors Journal*, vol. 21, no. 9, pp. 10 824–10 833, 2021.
- [111] E. Ayodele, S. Zaidi, J. Scott, Z. Zhang, A. Hayajneh, S. Shittu, and D. McLernon, "A weft knit data glove," *IEEE Transactions on Instrumentation and Measurement*, vol. 70, pp. 1–12, 2021.
- [112] Y. Zhang, Y. Huang, Y. Ge, and N. Bao, "A master–slave hand operation cooperative perception system for grasping object via information fusion of flexible strain sensors," *Measurement*, vol. 169, p. 108437, 2021.
- [113] Y.-T. Tsai, W.-Y. Jhu, C.-C. Chen, C.-H. Kao, and C.-Y. Chen, "Unity game engine: Interactive software design using digital glove for virtual reality baseball pitch training," *Microsystem Technologies*, vol. 27, no. 4, pp. 1401–1417, 2021.
- [114] M. A. Ahmed, B. Bahaa, A. Zaidan, M. Salih, Z. Al-qaysi, and A. Alamoodi, "Based on wearable sensory device in 3d-printed humanoid: A new real-time sign language recognition system," *Measurement*, vol. 168, p. 108431, 2021.

- [115] F. Fei, S. Xian, X. Xie, C. Wu, D. Yang, K. Yin, and G. Zhang, "Development of a wearable glove system with multiple sensors for hand kinematics assessment," *Micromachines*, vol. 12, no. 4, p. 362, 2021.
- [116] S. Lee, Y. Choi, M. Sung, J. Bae, and Y. Choi, "A knitted sensing glove for human hand postures pattern recognition," *Sensors*, vol. 21, no. 4, p. 1364, 2021.
- [117] Y. Li, H. Di, Y. Xin, and X. Jiang, "Optical fiber data glove for hand posture capture," *Optik*, vol. 233, p. 166603, 02 2021.
- [118] Z. Li, L. Cheng, and Q. Song, "An ultra-stretchable and highly sensitive photoelectric effect-based strain sensor: Implementation and applications," *IEEE Sensors Journal*, vol. 21, no. 4, pp. 4365–4376, 2020.
- [119] T. Muezzinoglu and M. Karakose, "An intelligent human-unmanned aerial vehicle interaction approach in real time based on machine learning using wearable gloves," *Sensors*, vol. 21, no. 5, p. 1766, 2021.
- [120] F. Santoni, A. De Angelis, A. Moschitta, and P. Carbone, "Magik: A hand-tracking magnetic positioning system based on a kinematic model of the hand," *IEEE Transactions on Instrumentation and Measurement*, vol. 70, pp. 1–13, 2021.
- [121] S. Shin, H. U. Yoon, and B. Yoo, "Hand gesture recognition using egain-silicone soft sensors," *Sensors*, vol. 21, no. 9, p. 3204, 2021.
- [122] J. Wang, B. Li, Z. Li, I. Zubrycki, and G. Granosik, "Grasping behavior of the human hand during tomato picking," *Computers and Electronics in Agriculture*, vol. 180, p. 105901, 2021.
- [123] G. Yuan, X. Liu, Q. Yan, S. Qiao, Z. Wang, and L. Yuan, "Hand gesture recognition using deep feature fusion network based on wearable sensors," *IEEE Sensors Journal*, vol. 21, no. 1, pp. 539–547, 2020.
- [124] L. Yuan, W. Qi, K. Cai, C. Li, Q. Qian, and Y. Zhou, "Gesture recognition device based on cross reticulated graphene strain sensors," *Journal of Materials Science: Materials in Electronics*, vol. 32, no. 7, pp. 8410–8417, 2021.
- [125] T. Simoes Dias, J. J. A. M. Junior, and S. F. Pichorim, "An instrumented glove for recognition of brazilian sign language alphabet," *IEEE Sensors Journal*, vol. 22, no. 3, pp. 2518–2529, 2022.
- [126] D. Dutta, S. Aruchamy, S. Mandal, and S. Sen, "Poststroke grasp ability assessment using an intelligent data glove based on action research arm test: Development, algorithms, and experiments," *IEEE Transactions on Biomedical Engineering*, vol. 69, no. 2, pp. 945–954, 2022.
- [127] M. Lee and J. Bae, "Real-time gesture recognition in the view of repeating characteristics of sign languages," *IEEE Transactions on Industrial Informatics*, vol. 18, no. 12, pp. 8818–8828, 2022.
- [128] J. Li, X. Liu, Z. Wang, T. Zhang, S. Qiu, H. Zhao, X. Zhou, H. Cai, R. Ni, and A. Cangelosi, "Real-time hand gesture tracking for human-computer interface based on multi-sensor data fusion," *IEEE Sensors Journal*, vol. 21, no. 23, pp. 26 642–26 654, 2021.
- [129] H. Sarwat, H. Sarwat, S. A. Maged, T. H. Emara, A. M. Elbokl, and M. I. Awad, "Design of a data glove for assessment of hand performance using supervised machine learning," *Sensors*, vol. 21, no. 21, p. 6948, 2021.
- [130] Y. Choi, S. Lee, M. Sung, J. Park, S. Kim, and Y. Choi, "Development of emg-fmg based prosthesis with pvdf-film vibrational feedback control," *IEEE Sensors Journal*, vol. 21, no. 20, pp. 23 597–23 607, 2021.
- [131] Q. Fu, J. Fu, S. Zhang, X. Li, J. Guo, and S. Guo, "Design of intelligent human-computer interaction system for hard of hearing and non-disabled people," *IEEE Sensors Journal*, vol. 21, no. 20, pp. 23 471–23 479, 2021.
- [132] E. Cazacu, C. van der Grinten, J. Bax, G. Baeten, F. Holtkamp, and C. Lee, "A position sensing glove to aid ankle-foot orthosis diagnosis and treatment," *Sensors*, vol. 21, no. 19, p. 6631, 2021.
- [133] A. H. Alrubayi, M. Ahmed, A. Zaidan, A. Albahri, B. Zaidan, O. Albahri, A. Alamoodi, and M. Alazab, "A pattern recognition model for static gestures in malaysian sign language based on machine learning techniques," *Computers & Electrical Engineering*, vol. 95, p. 107383, 2021.
- [134] S. M. Biju, H. Z. Sheikh, M. F. Malek, F. Oroumchian, and A. Bell, "Design of grip strength measuring system using FSR and flex sensors using SVM algorithm," *IAES International Journal of Artificial Intelligence (IJ-AI)*, vol. 10, no. 3, p. 676, 2021.
- [135] M. Ahmed, B. Zaidan, A. Zaidan, A. Alamoodi, O. Albahri, Z. Al-Qaysi, A. Albahri, and M. M. Salih, "Real-time sign language framework based on wearable device: analysis of msl, dataglove, and gesture recognition," *Soft Computing*, vol. 25, no. 16, pp. 11 101–11 122, 2021.
- [136] C. Wu, K. Wang, Q. Cao, F. Fei, D. Yang, X. Lu, B. Xu, H. Zeng, and A. Song, "Development of a low-cost wearable data glove for capturing finger joint angles," *Micromachines*, vol. 12, no. 7, p. 771, 2021.
- [137] J. Maitre, C. Rendu, K. Bouchard, B. Bouchard, and S. Gaboury, "Object recognition in performed basic daily activities with a handcrafted data glove prototype," *Pattern Recognition Letters*, vol. 147, pp. 181–188, 2021.
- [138] D. Sim, Y. Baek, M. Cho, S. Park, A. Sagar, and H. S. Kim, "Low-latency haptic open glove for immersive virtual reality interaction," *Sensors*, vol. 21, no. 11, p. 3682, 2021.
- [139] K. Guo, S. Zhang, S. Zhao, and H. Yang, "Design and manufacture of data gloves for rehabilitation training and gesture recognition based on flexible sensors," *Journal of Healthcare Engineering*, vol. 2021, 2021.
- [140] N. B. Gosala, F. Wang, Z. Cui, H. Liang, O. Glauser, S. Wu, and O. Sorkine-Hornung, "Self-calibrated multi-sensor wearable for hand tracking and modeling," *IEEE Transactions on Visualization and Computer Graphics*, pp. 1–1, 2021.
- [141] S. Davarzani, M. A. Ahmadi-Pajouh, and H. Ghafarirad, "Design of sensing system for experimental modeling of soft actuator applied for finger rehabilitation," *Robotica*, pp. 1–21, 2021.
- [142] X. Han, X. Miao, Q. Liu, Y. Li, and A. Wan, "A fabric-based integrated sensor glove system recognizing hand gesture," *Autex Research Journal*, vol. 0, no. 0, 2021.
- [143] A. Calado, V. Errico, and G. Saggio, "Toward the minimum number of wearables to recognize signer-independent italian sign language with machine-learning algorithms," *IEEE Transactions on Instrumentation and Measurement*, vol. 70, pp. 1–9, 2021.
- [144] Y. Dong, J. Liu, and W. Yan, "Dynamic hand gesture recognition based on signals from specialized data glove and deep learning algorithms," *IEEE Transactions on Instrumentation and Measurement*, vol. 70, pp. 1–14, 2021.
- [145] K. Aw, J. Budd, and T. Wilshaw-Sparkes, "Data glove using soft and stretchable piezoresistive sensors," *Micromachines*, vol. 13, no. 3, p. 372, 2022.
- [146] Y.-T. Hwang, W.-A. Lu, and B.-S. Lin, "Use of functional data to model the trajectory of an inertial measurement unit and classify levels of motor impairment for stroke patients," *IEEE Transactions on Neural Systems and Rehabilitation Engineering*, vol. 30, pp. 925–935, 2022.
- [147] H. Elwahsh, A. Elkhoully, E. A. Nasr, A. K. Kamrani, and E. El-shafei, "A new intelligent approach for deaf/dumb people based on deep learning," *CMC-COMPUTERS MATERIALS & CONTINUA*, vol. 72, no. 3, pp. 6045–6060, 2022.
- [148] D. W. O. Antillon, C. R. Walker, S. Rosset, and I. A. Anderson, "Glove-based hand gesture recognition for diver communication," *IEEE Transactions on Neural Networks and Learning Systems*, pp. 1–13, 2022.
- [149] Y. Wang and J. Sun, "Design and implementation of virtual reality interactive product software based on artificial intelligence deep learning algorithm," *Advances in Multimedia*, vol. 2022, 2022.
- [150] A. Boruah, N. M. Kakoty, T. Ali, and M. Malarvili, "Shape oriented object recognition on grasp using features from enclosure based exploratory procedure," *International Journal of Intelligent Robotics and Applications*, pp. 1–17, 2022.
- [151] A. Yudhana, I. C. Kurniawan, I. Anshori, and I. Mufandi, "Performance evaluation of communication methods on electric wheelchairs as assistive technology for persons with disabilities," *International Journal on Smart Sensing and Intelligent Systems*, vol. 15, no. 1, 2022.
- [152] P. Zhang, W. Li, Q. Zhang, X. Wang, G. Lin, W. Li, Y. Li, K. Zhang, and L. Huang, "Mass-produced flexible strain sensors based on dip-coating and water bath for human-computer interaction," *IEEE Sensors Journal*, vol. 23, no. 2, pp. 1497–1506, 2023.
- [153] S. Duan, J. Wang, Y. Lin, J. Hong, Y. Lin, Y. Xia, Y. Li, D. Zhu, W. Lei, W. Su *et al.*, "Highly durable machine-learned waterproof electronic glove based on low-cost thermal transfer printing for amphibious wearable applications," *Nano Research*, pp. 1–10, 2022.
- [154] F. Huang, J. Hu, X. Yan, and F. Meng, "High-linearity, ultralow-detection-limit, and rapid-response strain sensing yarn for data gloves," *Journal of Industrial Textiles*, vol. 51, no. 3\_suppl, pp. 4554S–4570S, 2022.



- [155] A. Maddahi, T. R. Leach, M. Saeedi, P. R. Dhannapuneni, Y. Maddahi, M.-A. Choukou, and K. Zareinia, "Roboethics in remote human interactions and rehabilitative therapeutics," *Applied Sciences*, vol. 12, no. 12, p. 6033, 2022.
- [156] T. Bright, S. Adali, and G. Bright, "Low-cost sensory glove for human-robot collaboration in advanced manufacturing systems," *Robotics*, vol. 11, no. 3, p. 56, 2022.
- [157] S. Kerner, M. Krugh, and L. Mears, "Wearable shear and normal force sensing glove development for real-time feedback on assembly line processes," *Journal of Manufacturing Systems*, vol. 64, pp. 668–675, 2022.
- [158] H. Zhou, T. Lu, Y. Liu, S. Zhang, and M. Gowda, "Learning on the rings: Self-supervised 3d finger motion tracking using wearable sensors," *Proceedings of the ACM on Interactive, Mobile, Wearable and Ubiquitous Technologies*, vol. 6, no. 2, pp. 1–31, 2022.
- [159] W. Zheng, N. Guo, B. Zhang, J. Zhou, G. Tian, and Y. Xiong, "Human grasp mechanism understanding, human-inspired grasp control and robotic grasping planning for agricultural robots," *Sensors*, vol. 22, no. 14, p. 5240, 2022.
- [160] B. Anbalagan, S. Karnam Anantha, and R. Kalpana, "Novel approach to prognosis parkinson's disease with wireless technology using resting tremors," *Wireless Personal Communications*, vol. 125, no. 4, pp. 2985–2999, 2022.
- [161] S. Elksass, H. A. Alkabes, N. M. El-Kemary, K. E. El-Kelany, and M. El-Kemary, "Anti-bacterial and multi-functional smart wearable sensor based on organo-hydrogel for diagnosis of the anterior cruciate ligament injuries, and sensing glove for rehabilitation of joints motion," *Materials Today Communications*, vol. 32, p. 104131, 2022.
- [162] J. Piskozub and P. Strumillo, "Reducing the number of sensors in the data glove for recognition of static hand gestures," *Applied Sciences*, vol. 12, no. 15, p. 7388, 2022.
- [163] W. Lin, C. Li, and Y. Zhang, "Interactive application of data glove based on emotion recognition and judgment system," *Sensors*, vol. 22, no. 17, p. 6327, 2022.
- [164] A. Calado, P. Roselli, V. Errico, N. Magrofuoco, J. Vanderdonck, and G. Saggio, "A geometric model-based approach to hand gesture recognition," *IEEE Transactions on Systems, Man, and Cybernetics: Systems*, vol. 52, no. 10, pp. 6151–6161, 2022.
- [165] S. M. Biju and H. Z. Sheikh, "Sensor evaluation for hand grip strength," *International Journal of Electrical & Computer Engineering (2088-8708)*, vol. 12, no. 5, 2022.
- [166] J. DelPreto, J. Hughes, M. D'Aria, M. de Fazio, and D. Rus, "A wearable smart glove and its application of pose and gesture detection to sign language classification," *IEEE Robotics and Automation Letters*, vol. 7, no. 4, pp. 10589–10596, 2022.
- [167] Y. Zhang, W. Xu, X. Zhang, and L. Li, "Sign annotation generation to alphabets via integrating visual data with somatosensory data from flexible strain sensor-based data glove," *Measurement*, vol. 202, p. 111700, 2022.
- [168] B.-S. Lin, I.-J. Lee, P.-C. Hsiao, S.-Y. Yang, C.-Y. Chen, S.-H. Lee, Y.-F. Huang, M.-H. Yen, and Y. H. Hu, "Design of a multi-sensor system for exploring the relation between finger spasticity and voluntary movement in patients with stroke," *Sensors*, vol. 22, no. 19, p. 7212, 2022.
- [169] T. Cerqueira, F. M. Ribeiro, V. H. Pinto, J. Lima, and G. Gonçalves, "Glove prototype for feature extraction applied to learning by demonstration purposes," *Applied Sciences*, vol. 12, no. 21, p. 10752, 2022.
- [170] A. Hekmat, Z. Zuping, and H. S. S. Al-deen, "Map modeling for full body gesture using flex sensor and machine learning algorithms," *Multimedia Systems*, pp. 1–16, 2022.
- [171] S. Sadhu, D. Solanki, N. Constant, V. Ravichandran, G. Cay, M. J. Saikia, U. Akbar, and K. Mankodiya, "Towards a telehealth infrastructure supported by machine learning on edge/fog for parkinson's movement screening," *Smart Health*, vol. 26, p. 100351, 2022.
- [172] A. A. Zakri, A. H. Arfianti Arfianti, M. Iqbal, H. Madjid, and N. F. Aulia, "Designing flex sensor gloves with temperature sensor & pulse sensor to help stroke patients," *International Journal of Emerging Technology and Advanced Engineering*, vol. 12, pp. 23–31, 2022.
- [173] C. Yu, S. Fan, Y. Liu, and Y. Shu, "End-side gesture recognition method for uav control," *IEEE Sensors Journal*, vol. 22, no. 24, pp. 24526–24540, 2022.
- [174] Y. Liao, Y. Cheng, Z. Zhuang, R. Li, Y. Yu, R. Wang, and Z. Jiao, "Plasma-sprayed flexible strain sensor and its applications in boxing glove," *Applied Sciences*, vol. 12, no. 16, p. 8382, 2022.
- [175] H. Huang, Z. Liang, F. Sun, M. Dong *et al.*, "Virtual interaction and manipulation control of a hexacopter through hand gesture recognition from a data glove," *Robotica*, vol. 40, no. 12, pp. 4375–4387, 2022.
- [176] Y. Luo, X. Chen, X. Li, H. Tian, S. Li, L. Wang, J. He, Z. Yang, and J. Shao, "Heterogeneous strain distribution based programmable gated microchannel for ultrasensitive and stable strain sensing," *Advanced Materials*, p. 2207141, 2022.
- [177] T. S. Dias, J. J. A. M. Junior, and S. F. Pichorim, "Comparison between handcraft feature extraction and methods based on recurrent neural network models for gesture recognition by instrumented gloves: A case for brazilian sign language alphabet," *Biomedical Signal Processing and Control*, vol. 80, p. 104201, 2023.
